# Supplementary material for: Sem4SAP: Synonymous Expression Mining From Open Knowledge Graph For Language Model Synonym-Aware Pretraining
Source: arXiv:2303.14425 source file (2023-03-25)
Supplement: Supplementary file 1 [file 09_Appendix.tex]

\begin{table*}[!t]
    \small
    \centering
    \resizebox{\textwidth}{!}{
    \begin{tabular}{|c|c|c|c|c|c|c|}
        \hline
        \textbf{Dataset} & \textbf{Language} & \textbf{Task Type} & \textbf{\#Labels} & \textbf{\#Train} & \textbf{\#Validation} & \textbf{\#Test}\\
        \hline
        \hline
        SST & English & Classification & 2 & 67350 & 873 & 1822\\
        \hline
        MRPC & English & Classification & 2 & 3669 & 409 & 1726\\
        \hline
        QQP & English & Classification & 2 & 363871 & 40432 & 390965\\
        \hline
        MNLI-mm & English & Classification & 3 & 392703 & 9832 & 9847\\
        \hline
        RTE & English & Classification & 2 & 2491 & 278 & 3001\\
        \hline
        \hline
        AFQMC & Chinese & Classification & 2 & 34334 & 4316 & 3861\\
        \hline
        TNEWS & Chinese & Classification & 15 & 53360 & 10000 & 10000\\
        \hline
        IFLYTEK & Chinese & Classification & 119 & 12133 & 2599 & 2600\\
        \hline
        CMNLI & Chinese & Classification & 3 & 391783 & 12426 & 13880\\
        \hline
        CSL & Chinese & Classification & 2 & 20000 & 3000 & 3000\\
        \hline
    \end{tabular}
    }
    \vspace{-2mm}
    \caption{Statistics information about the datasets we used in experiments.}
    \vspace{-5mm}
    \label{tab: datasets}
\end{table*}

We elaborate the datasets we used in experiment in this section, 
and the statistics are listed in Table~\ref{tab: datasets}.
\begin{itemize}
    \item SST~\cite{socher2013sst}: The Stanford Sentiment Treebank consists of sentences from movie reviews and human annotations of their sentiment. The task is to predict the sentiment of a given sentence in the two-way (positive/negative) class split.
    \item MRPC~\cite{dolan2005mrpc}: The Microsoft Research Paraphrase Corpus is a corpus of sentence pairs automatically extracted from online news sources, with human annotations for whether the sentences in the pair are semantically equivalent.
    \item QQP~\footnote{https://www.quora.com/profile/Ricky-Riche-2/First-Quora-Dataset-Release-Question-Pairs}: The Quora Question Pairs (QQP) dataset is a collection of question pairs from the community question-answering website Quora. The task is to determine whether a pair of questions are semantically equivalent.
    \item MNLI~\cite{williams2017mnli}: The Multi-Genre Natural Language Inference Corpus is a crowdsourced collection of sentence pairs with textual entailment annotations. Given a premise sentence and a hypothesis sentence, the task is to predict whether the premise entails the hypothesis (entailment), contradicts the hypothesis (contradiction), or neither (neutral).
    \item RTE~\cite{dagan2006rte1}: The Recognizing Textual Entailment datasets come from a series of annual textual entailment challenges. Examples are constructed based on news and Wikipedia text. The dataset convert all datasets to a two-class split, where for three-class datasets the dataset collapse neutral and contradiction into not entailment, for consistency.
    \item AFQMC~\footnote{https://dc.cloud.alipay.com/index/\#/topic/intro?id=3}: The Ant Financial Question Matching Corpus comes from Ant Technology Exploration Conference Developer competition. It is a binary classification task that aims to predict whether two sentences are semantically similar
    \item TNEWS~\footnote{https://github.com/aceimnorstuvwxz/toutiao-text-classfication-dataset}: TouTiao Text Classification for News Titles consists of Chinese news published by TouTiao. The task is to predict which category the title belongs to. 
    \item IFLYTEK: IFLYTEK is constructed by IFLYTEK CO., which contains 17,332 app descriptions. The task is to assign each description into one of 119 categories, such as food, car rental, education, etc. 
    \item CMNLI: The CMNLI data consisted of two parts: XNLI~\cite{conneau2018xnli} and MNLI~\cite{williams2017mnli}. This dataset can be used to determine whether a given two sentences are in an implicative, neutral, or contradictory relationship with each other. 
    \item CSL~\cite{li2022csl}: Chinese Scientific Literature dataset contains Chinese paper abstracts and their keywords from core journals of China, covering multiple fields of natural sciences and social sciences. The task is to tell whether the keywords are all original keywords of a paper when given an abstract and some keywords.
\end{itemize}
